# Supplementary material for: Distributed Estimation, Control and Coordination of Quadcopter Swarm Robots
Source: arXiv:2102.07107 source file (2021-02-14)
Supplement: Supplementary file 1 [file appendix.tex]

\chapter{Something}\label{sec:something}

Blah, blah \dots

 \cleardoublepage

\chapter{Again Something}\label{sec:again_something}

Blah, blah \dots

 \cleardoublepage
